# Supplementary material for: Enhanced 3D Urban Scene Reconstruction and Point Cloud Densification using Gaussian Splatting and Google Earth Imagery
Source: arXiv:2405.11021 source file (2024-06-01)
Supplement: Supplementary file 1 [file 12_appendix.tex]

\section{Appendix Section}
\label{sec:appendix_section}
Supplementary material goes here.
